# Supplementary material for: Quenching, bursting and galaxy shapes: colour transformation as a function of morphology
Source: arXiv:2111.11450 source file (2021-11-22)
Supplement: Supplementary file 1 [file Appendix.tex]

\label{Appendix}
%%%%%%%%%%%%%%%%%%%%%%%%%%%%%%%%%%%%%%%%%%%%%%%%%%%%%%%%%%%%%%%%%%%%%%%%%%%%%%%%%%%%%%%%%%%%%%
Here we present the $\Delta(NUV-r)_0=0.5$ binned data used in Figure \ref{fig_sfa_moneyplot}. For Table \ref{tab_stats_dl} we have:

\begin{itemize}
    \item \textsuperscript{a}: binned sample size, for ellipticals and spirals;
    \item \textsuperscript{b}: binned $(NUV-r)_0$ average value, for ellipticals and spirals;
    \item \textsuperscript{c}: binned SFA average, for ellipticals and spirals;
    \item \textsuperscript{d}: Permutation estimated by Monte Carlo $p-value$
\end{itemize}{}
